# Supplementary material for: Scaling Superconducting Quantum Computers with Chiplet Architectures
Source: arXiv:2210.10921 source file (2022-10-19)
Supplement: Supplementary file 1 [file 9Appendix.tex]

\section{Appendix}
